# Supplementary material for: A Finite-State Controller Based Offline Solver for Deterministic POMDPs
Source: arXiv:2505.00596 ancillary file (2025-05-01)
Supplement: Supplementary file 1 [file supp.pdf]

# Appendix: A Finite-State Controller Based Offline Solver for Deterministic POMDPs

**Alex Schutz**[1], **Yang You**[2], **Matias Mattamala**[1], **Ipek Caliskanelli**[2], **Bruno Lacerda**[1] and **Nick Hawes**[1]

[1]University of Oxford

[2]UK Atomic Energy Authority

{alexschutz, matias, bruno, nickh}@robots.ox.ac.uk, {yang.you, ipek.caliskanelli}@ukaea.uk

## MCVI Algorithm

Algorithm A1 contains the procedure for the backup process of the original MCVI algorithm. The algorithm is presented using a discounted-reward formulation for a POMDP, where $R(s, a)$ is the reward given by taking action $a$ in state $s$, and $\gamma < 1$ is the discount factor.

**Algorithm A1:** MCVI Backup

**Function** MCVI BACKUP($F = \langle \mathcal{V}, \eta, \psi \rangle, b, N, k$)
- For each action $a \in \mathcal{A}$, $R_a \leftarrow 0$.
- For each action $a \in \mathcal{A}$, each observation $o \in \mathcal{O}$, and each node $v \in \mathcal{V}$, $V_{a,o,v} \leftarrow 0$.
- **for** each action $a \in \mathcal{A}$ **do**
  - **for** $i = 1$ to $N$ **do**
    - $s_i \leftarrow s \sim b$.
    - $s'_i \leftarrow s' \sim \Pr(s'_i | s_i, a)$.
    - $o_i \leftarrow o \sim \Pr(o_i | s'_i, a)$.
    - $R_a \leftarrow R_a + R(s_i, a)$.
    - **for** each node $v \in \mathcal{V}$ **do**
      - Calculate $\alpha_{F,v}(s'_i)$ via $k$ rollouts of the policy $\pi_{F,v}$.
      - $V_{a,o_i,v} \leftarrow V_{a,o_i,v} + \alpha_{F,v}(s'_i)$.
  - **for** each observation $o \in \mathcal{O}$ **do**
    - $V_{a,o} \leftarrow \max_{v \in \mathcal{V}} V_{a,o,v}$.
    - $v_{a,o} \leftarrow \arg\max_{v \in \mathcal{V}} V_{a,o,v}$.
  - $V_a \leftarrow (R_a + \gamma \sum_{o \in \mathcal{O}} V_{a,o})/N$.
- $V^{F'} \leftarrow \max_{a \in \mathcal{A}} V_a$.
- $a^\star \leftarrow \arg\max_{a \in \mathcal{A}} V_a$.
- Create a new FSC $F' = \langle \mathcal{V}', \eta', \psi' \rangle$. Set $\psi'(v'_0) = a^\star$ and $\eta'(v'_0, o) = v_{a^\star,o}$. For $k \in 1, \ldots, |\mathcal{V}|$, set $\psi'(v'_k) = \psi(v_{k-1})$ and $\eta'(v'_k, o) = \eta(v_{k-1}, o)$.
- **return** $F'$

## Algorithm Implementation

All algorithms were implemented by the authors in C++ except SARSOP, where we use the model to create an input file suitable for the C++ implementation made available by Kurniawati *et al.* [2009]. As SARSOP is designed for use with discounted infinite-horizon problems, we use a discount factor $\gamma = 0.01^{1/T}$. All planning was executed on a single core of a 4.8 GHz 12th Gen Intel Core i7-12800H processor with 32GB memory.

## Algorithm Code

Code for the the DetMCVI implementation can be found at http://github.com/ori-goals/DetMCVI.

## Algorithm Parameters

We present the parameters used in the paper to evaluate the performance of each algorithm on the set of deterministic POMDP problems in Table A1, with problem-varying parameters presented in Table A2.

## Domain Descriptions

**Canadian Traveller Problem** We implement the CTP as described in Example 1, illustrated in Figure 3a. In order to guarantee reachability of the goal state, we add a special action to transition to the goal state, which is only valid when the goal node is not reachable from the start node under the edge configuration of the initial state. Following Aksakalli *et al.* [2016], problem sets for the CTP were constructed using $n$ randomly generated points within a $100 \times 100$ grid, with edges connecting points according to a Delaunay triangulation. Of these edges, 25% were randomly selected to be stochastic edges, each with a blockage probability sampled from the standard uniform distribution. Origin and goal nodes were chosen to be the most distant points in the map. We set $T = 2n$. Each problem set contains 10 different CTP instances of the same $n$.

**Wumpus** An agent moves around a maze, where one tile contains gold, one tile contains a Wumpus, and some tiles contain pits with a 20% chance [Russell and Norvig, 2021]. Two goal states are possible: the agent moves into a tile containing a pit or the Wumpus, associated with a high cost, or the agent climbs out at the entrance after picking up the gold, associated with a low cost. A breeze indicates a pit in one of the adjacent tiles, and a stench indicates the presence of an adjacent Wumpus. The player starts with an arrow which can be used to remove the Wumpus if it is in the path of the shot. An example of the problem is shown in Figure 3b. We

| Algorithm | Parameter | Value |
|---|---|---|
| General | Maximum policy node count | 3125000 |
| | Evaluation trial count | 10000 |
| | Evaluation interval | Problem varying |
| | Maximum planning time | Problem varying |
| | Horizon | Problem varying |
| DetMCVI | Convergence threshold | 0.005 |
| | Initial belief sample size | 100000 |
| | Maximum belief size | 10000 |
| MCVI | Convergence threshold | 0.005 |
| | Initial belief size | 10000 |
| Q-Learning | Learning rate | 0.9 |
| | Decay factor | 0.01 |
| | Initial $\epsilon$ | 1 |
| | Final $\epsilon$ | 0.1 |
| | Simulation depth | 15 |
| | Episode size | 30 |
| | Episode count | 10 |
| | Simulations per trial | 40 |
| | Convergence threshold | 0.001 |
| Anytime AO$^\star$ | Probability of OUT node | 0.5 |
| SARSOP | Precision | 0.005 |
| | Trial improvement factor | 0.5 |

Table A1: Parameters used for baseline evaluation of different deterministic POMDP problems

evaluate Wumpus grid worlds of size $n \times n$ for $n = 2,\ 3,\ 4,$ imposing a horizon of $50n$.

**Maze** Shown in Figure 3c, an agent is located in a square grid maze with a fixed goal location. The starting position and orientation of the agent is uniformly distributed over each non-goal location. The agent can observe only the 4-connected walls, and can move forward one square or turn left, right, or around, at a cost of 1. We set $T = 8n^2 + 4n$, where $n$ is the number of rows in the maze. Problem sets for the Maze World were constructed using 10 randomly generated mazes of the same $n$, where $n$ is the number of rows/columns in the maze.

**Sort** The state consists of a list of $n$ numbers, as shown in Figure 3d, with the goal state being reached when the list is sorted in ascending order. Actions are to swap any pair of numbers for a cost of 10, and the received observation is the Spearman footrule distance between the new state and the goal state. We impose a horizon of $T = 2n$.

## Belief Sampling Method

DetMCVI operates on a sample of a belief, which we represent using a probability mass function (pmf), describing the states in the support of the belief and their probabilities:

$$\text{pmf}_b = \{(s_i, p_i) \mid s_i \in \text{Supp}(b),\ p_i > 0,\ \sum_i p_i = 1\}.$$

To generate a pmf which approximates $b_0$, we take $10N$ samples of $b_0$, thus constructing $\text{pmf}_{\tilde{b_0}}$. The induced belief, $\tilde{b_0}$ may have up to $10N$ states in $\text{Supp}(\tilde{b_0})$. We seek to limit the maximum number of states in the support of the initial belief used for planning to $N$ states, thus we will construct a downsampled belief $\tilde{\tilde{b}}$.

To achieve this, we perform a weighted shuffle. Let $E_i \sim \text{Exponential}(\lambda = 1)$, and compute $w_i = \frac{E_i}{p_i}$ for each probability $p_i$ in $\text{pmf}_{\tilde{b_0}}$. Find an ordering $j$ such that $w_{j_1} \leq w_{j_2} \leq \ldots \leq w_{j_n}$. This allows us to sort the list of $(s_i, p_i)$ pairs in ascending order:

$$\{(s_{j_1}, p_{j_1}), (s_{j_2}, p_{j_2}), \ldots, (s_{j_n}, p_{j_n})\}.$$

From this ordering, we construct a downsampled pmf:

$$\text{pmf}_{\tilde{\tilde{b}}} = \left\{ \left( s_{j_k}, \frac{p_{j_k}}{\eta} \right) \mid k = 1, \ldots, N \right\},$$

where $\eta$ is a normalising constant.

## Shortest Path Calculation

For DetMCVI, AO$^\star$, and QMDP Trees, the lower bound heuristic is given by the full observability relaxation of the DetPOMDP. Due to the deterministic transition function, this simply requires finding the shortest path to a goal state from each state in the belief, where states are nodes and transitions are edges. As we only assume sample-based access to the transition function, we can only easily enumerate the outgoing edges of a node (finding the incoming edges requires iterating over the entire state space). This means that we must solve a single-source shortest path problem and choose the

| Domain | $n$ | Max planning time (s) | Evaluation interval (s) | Horizon |
|---|---|---|---|---|
| CTP | 20 | 3600 | 1 | 40 |
| | 50 | 2700 | 120 | 100 |
| | 100 | 36000 | 1200 | 200 |
| Wumpus | 2 | 120 | 0.5 | 100 |
| | 3 | 1200 | 6 | 150 |
| | 4 | 18000 | 600 | 200 |
| Maze | 10 | 1200 | 4 | 420 |
| | 15 | 14400 | 200 | 930 |
| | 20 | 36000 | 600 | 1640 |
| Sort | 5 | 140 | 1 | 10 |
| | 7 | 18000 | 200 | 14 |

Table A2: Problem-varying parameters for each domain

best goal state for each state in the belief. In addition, shortest paths may be restricted by the horizon of the problem. For our implementation we use the Bellman-Ford algorithm with an additional restriction on depth.

Note that if we had access to the transition function, we could solve the single-destination shortest path problem for the goal state by reversing the edge directions, eliminating repeated calculations. However, in practice, the transition function for many domains we are interested in is too large to fit into memory.

## Forest Experiment Description

An area of a forest is surveyed by an ANYbotics ANYmal D. The paths generated by the survey method are designed to maximise the coverage of the forest area, and retracing the path of the robot to return home would take much longer than finding a more direct route. A topological map is created using the traversed paths. From this map, we add "shortcut" edges between nodes to increase the connectivity of the map and provide a shorter route home. Since these added edges have not been previously traversed, the blockage probability of the new edge is estimated from the terrain data. The resultant graph is a form of the CTP. In this domain, the robot is cannot discern edge status by reaching a node, but must attempt to traverse an edge in order to establish its status, returning to the previous node if the edge is impassable.

We use a connected section of the topological map generated from operator-guided traversal through a forest using a LIDAR-based SLAM system. Shortcut edges are added if their addition results in at least a 25% reduction in Euclidean path length between two points, alongside a basic obstacle check using the point cloud. Edge costs are the Euclidean distance between the points in metres. Figure A1 shows the map used, with added shortcut edges highlighted. A set of 50 problem instances were generated by randomly selecting blockage probabilities for the shortcut edges, and randomly choosing points for the origin and goal nodes, provided they were at least 25 metres apart in the topological map. The planning budget was set to 300 seconds.

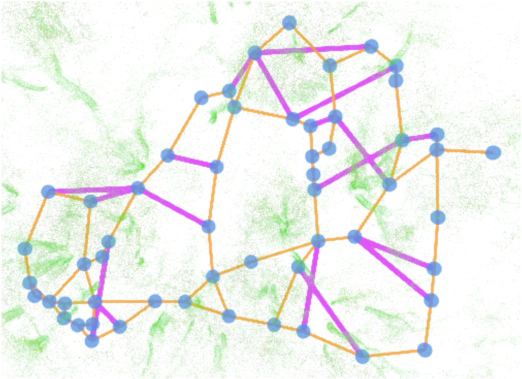

Figure A1: Topological map of a section of a forest, overlaid with recorded point cloud. Operator-navigated edges are shown in orange and shortcuts added via post-processing are highlighted in purple.

## References


[Aksakalli *et al.*, 2016] Vural Aksakalli, O Furkan Sahin, and Ibrahim Ari. An AO* based exact algorithm for the Canadian traveler problem. *INFORMS Journal on Computing*, 28(1):96–111, 2016.

[Kurniawati *et al.*, 2009] Hanna Kurniawati, David Hsu, and Wee Sun Lee. SARSOP: Efficient Point-Based POMDP Planning by Approximating Optimally Reachable Belief Spaces. 2009.

[Russell and Norvig, 2021] S. Russell and P. Norvig. *Artificial Intelligence: A Modern Approach, Global Edition*. Pearson Education, 2021.
